# Supplementary material for: Types are Internal $\infty$-Groupoids
Source: arXiv:2105.00024 source file (2021-04-30)
Supplement: Supplementary file 1 [file appendix.tex]

\section{Proofs}

\begin{lem}[Strong confluence for the \ref{rewrite:muetar}/\ref{rewrite:mumu} pair]
  \label{proof:muetarmumu-proof}
  We fix a monad $M$ and show that the two rules can always be joined:
  if $t \leadsto_{\text{\ref{rewrite:muetar}}} t'$ and 
  $t \leadsto_{\text{\ref{rewrite:mumu}}} t''$
  then $t'' \leadsto^* t'$.
\end{lem}

\begin{proof}
  In case of overlap, the first application reduces in one step:
  \begin{align*}
    \upmu&\ (\upmu\ c\ \delta)\ (\lambda\ p \to \upeta\ (\Typ (\upmu\ c\ \delta)\ p)) \leadsto_{\text{\ref{rewrite:muetar}}} \upmu\ c\ \delta
  \end{align*}

  We show that applying the \ref{rewrite:mumu} rule instead results in the same term,
  where only one rule applies on a given subterm at each step:
  \begin{align*}
    \upmu&\ (\upmu\ c\ \delta)\ (\lambda\ p \to \upeta\ (\Typ (\upmu\ c\ \delta)\ p)) \leadsto_{\text{\ref{rewrite:mumu}},\beta} \\
    &\upmu\ c\ (\lambda\ p \to \upmu\ (\delta\ p)\ 
        (\lambda\ q \to \upeta\ (\Typ (\upmu\ c\ \delta)~(\mupos\ p\ q)))) \\
    &\leadsto_{\text{\ref{rewrite:muTyp}}} \upmu\ c\ (\lambda\ p \to \upmu\ (\delta\ p)\ 
        (\lambda\ q \to \\
        &\quad\quad \upeta\ (\Typ (\delta\ (\muposfst c\ \delta\ (\mupos\ p\ q)))\\
        &\quad\quad (\mupossnd c\ \delta\ (\mupos\ p\ q)))))\\
    &\leadsto_{\text{\eqref{rewrite:muposfst},\ref{rewrite:mupossnd}}}\\
    &\quad\quad\upmu\ c\ (\lambda\ p \to \upmu\ (\delta\ p)\
        (\lambda\ q \to \upeta\ (\Typ (\delta\ p)\ q)))\\
    &\leadsto_{\text{\ref{rewrite:muetar}}}\upmu\ c\ (\lambda\ p \to \delta\ p))) \leadsto_{\eta} \upmu\ c\ \delta
  \end{align*}  
\end{proof}

\begin{thm-apdx}{Theorem \ref{thm:slice-alg}}
  Let $(M \,, M\da)$ be a monad extension.  Then slice extension
  $(M_1 \,, M\da_1)$ is algebraic.
\end{thm-apdx}

\begin{proof}
  Unfolding the definitions, we have that $\Idx M_1$ is the
  iterated sum:
  \begin{equation}
    \label{eq:slc-idx}
    \begin{aligned}
      &\sum_{(i : \Idx M)} \sum_{(j : \Idxd M\da\, i)} 
      \sum_{(c : \Cns M\, i)} \\
      &\hspace{1cm} (p : \Pos M c) \to \Idxd M\da\, (\Typ M\, c\, p)
    \end{aligned}
  \end{equation}
  and for a given $(i,j,c,\nu)$, the type
  $\Idxd M\da_1\, (i,j,c,\nu)$ of dependent indices is itself an
  iterated sum of the form:
  \begin{align*}
    \sum_{(j : \Idxd M\da\, i)} \sum_{(r : j \equiv j')} 
    \sum_{(d : \Cnsd M\da\, c)} \Typd M\da\, d\ \equiv \nu
  \end{align*}
  In other words, if the tuple $(i,j,c,\nu)$ is seen as a constructor
  in $c$ with inputs and output decorated by elements of $\Idxd M\da$,
  then a element $(j',r,d,\tau)$ lying over it is simply a constructor
  of the dependent monad $M\da$ over $c$ whose intrinsic typing
  information (that is, indices assigned by the underlying dependent
  polynomial of $M\da$) matches the decoration of $c$.

  The constructors follow a similar pattern, but now assembled into
  trees: a constructor of the base monad $M_1$ is a tree $\sigma$
  whose internal nodes carry the additional information of a
  decoration of their incoming and outgoing edges  by
  elements of $\Idxd M\da$.  A constructor of $M\da_1$ lying over
  $\sigma$ is itself a tree $\sigma\da$ built from dependent
  constructors of $M\da$, and carrying the additional information of
  equalities witnessing that the typing information of each node
  agrees with the decoration of the node it lies over in $\sigma$, in
  the sense of the previous paragraph. 

  Now, the situation of the theorem is the following: we are given a
  4-tuple $(i,j,c,\nu) : \Idx M_1$ and a tree
  $\sigma : \Cns M_1\, (i,j,c,\nu)$ together with a decoration of this
  tree $\phi$ which assigns to each of the positions of $\sigma$, that
  is, to each of its nodes, an index living in $\Idxd M\da_1$, which
  as we have seen, means a single dependent constructor together with
  proofs that its typing information matches the local decoration of
  the node in $\sigma$. To prove the theorem, we must produce in this
  situation three pieces of data:
  \begin{itemize}
  \item An index $\omega : \Idxd M\da_1 (i,j,c,\nu)$
  \item A dependent tree $\sigma\da : \Cnsd M\da_1\, \omega$
  \item A proof that $\zeta : \Typd M\da_1\, \sigma\da\, \equiv \phi$
  \end{itemize}
  And moreover, we must show that the space of all such data is
  contractible.

  We will construct this data by induction on the tree $\sigma$.  In
  the case that $\sigma = \lf (i \,, j)$  we have necessarily that
  $c = \upeta\, M\, i$ and $\nu = \etadec j$, and we may take
  \begin{align*}
    \omega &= (j \,, \refl\, , \upetad\, M\da\, j \, , \etadecd \refl) \\
    \sigma\da &= \lfd\, (j \, , \refl) \\
    \zeta &= \mathsf{funext}\, \botelim
  \end{align*}

  For the inductive case, that is, when
  $\sigma = \nd c\, \delta\, \epsilon$, evaluating the decoration
  $\phi$ on the
  position corresponding to the base of our tree, that is
  $\phi\, (\inl \ttt)$, we obtain a 4-tuple $(j',r,d,\tau)$ where
  $j' : \Idxd M\da\, i$, $r : j' \equiv j$, $d : \Cnsd M\da\, c\, j'$ and
  $\tau : \Typd M\da d \equiv \nu$.  Then we define
  \begin{align*}
    \omega &= (j' \,, r \,, \upmud M\da\, d\, \delta\da' \,, \tau') \\
    \sigma\da &= \ndd (d \,, \tau)\, (\lambda p \to \delta\da' \, p \,, \tau'\, p \, q) \, \epsilon\da' \\
    \zeta &= \beta \cdot \zeta'
  \end{align*}
  in which the decorations $\delta\da'$ and $\epsilon\da'$, as well as
  the typing compatibilities $\tau'$ and $\zeta'$ are obtained from
  the induction hypothesis, and $\beta$ is a coherence asserting that
  the typing information of a constructor is unchanged when it is
  transported along an equality of indices.

  In summary: the decoration $\phi$ assigns to each node of the tree
  $\sigma$ a dependent constructor lying over the constructor
  occupying that node, together with compatibility information about
  the typing.  By induction on $\sigma$, we accumulate these dependent
  constructors into dependent tree $\sigma\da$ lying over $\sigma$,
  and at the same time accumulate witnesses that the typing of the
  nodes in the resulting tree agrees with $\phi$, which it clearly
  does by construction.
  
  To show uniqueness, we need to see that any other triple
  $(\omega',\sigma\da',\zeta')$ is equal to the one defined above.
  The proof again proceeds by induction on the given tree $\sigma$,
  and the crucial point is that all the data of this 3-tuple can be
  eliminated away.  To see this, let us expand
  $\omega' = (j',r,d,\tau)$.  Now, $r : j' \equiv j$, so we may
  eliminate and assume $j' = j$. Similarly,
  $\zeta' : \Typd M\da_1 \sigma\da' \equiv \phi$ is just an equality
  between the typing function for $\sigma\da'$ and the original
  decoration $\phi$.  Since $\phi$ was a free parameter to begin with,
  we can freely eliminate $\zeta'$ at this point and assume that
  $\phi$ actually \emph{is} typing function $\sigma\da'$.  We are left
  with just the dependent tree $\sigma\da'$ and the remaining two
  elements of $\omega'$, namely $(d, \tau)$.  But now, as we proceed
  by induction on $\sigma$, we can \emph{also} proceed by induction on
  the dependent tree $\sigma\da'$.  And in fact, this completely
  forces the values of $(d, \tau)$ via the indexing of dependent
  trees: for example, when $\sigma = \lf (i \,, j)$, the only valid
  possibility for $\sigma\da'$ is $\lfd (j \,, \refl)$, and in this
  case, we necessarily have
  $(d,\tau) = (\upetad M\da (j \,, \refl) \,, \etadecd \refl)$ as
  required. The $\nd$ case is similar, even if the path algebra is
  considerably more involved.
\end{proof}

\begin{thm-apdx}{Theorem \ref{thm:slice-unique}}
  Suppose $(M , M\da)$ is a monad extension and $X : \OpType M$
  an opetopic type such that $\Rel X$ is fibrant.  Moreover,
  suppose we are given the data of
  \begin{itemize}
  \item An equivalence $e_0 : (i : \Idx M) \to \Idxd M\da\, i \simeq X_0\, i$
  \item An equivalence $e_1 : (i : \Idx M_1) \to \Idxd M\da_1 \simeq_{e_0} X_1$ over $e_0$
  \item Proofs that $s : \upetad M\da \equiv_{e_0 , e_1} \upeta\alg_{m_2}$ and $t : \upmud M\da \equiv_{e_0 , e_1} \upmu\alg_{m_2}$    
  \end{itemize}
  Then there is an equivalence of opetopic types
  \[ X \simeq_{o} \OvrOpType M\, M\da \]
\end{thm-apdx}

\begin{proof}
  The proof is by coinduction, and so it suffices to produce elements
  $e_0', e_1', s', t'$ whose types are the same as those of the
  corresponding elements in the hypotheses, but modified by the
  transformations
  \begin{align*}
    (M , M\da) &\quad \mapsto \quad (M_1 , M\da_1) \\
    X &\quad \mapsto  \quad \Rel X
  \end{align*}
  Next, we observe that it follows from univalence that the
  equivalences $e_0$ and $e_1$ can be eliminated from the hypotheses
  since the opetopic type $X$ is abstract. In other words, we are free
  to assume that $X_0 = \Idxd M\da$ and $X_1 = \Idxd M\da_1$ so that
  the first remaining abstract family of $X$ is
  \[ X_2 : \Idx M_2 \to \UU \] Moreover, after making these
  simplifications, the equalities $s$ and $t$ take the following
  types:
  \begin{align*}
    &s : (i : \Idx PM)\, (j : \Idxd PM\da i) \\
    &\hspace{.3cm} \to (j , \upetad PM\da\, j) \equiv \upeta\alg_{m_2}\, (\fst i)\, (\snd i) \\
    \\
    &t : (i : \Idx PM)\, (c : \Cns PM i) \\
    &\hspace{.3cm} \to (\delta : \Pos PM\, c) \to \Cns PM\, (\Typ PM\, c\, p) \\
    &\hspace{.3cm} \to (j : \Idxd PM\da\, i) (d : \Cnsd PM\da\, j\, c) \\
    &\hspace{.3cm} \to (\delta\da : (p : \Pos PM\, c) \to \Cnsd PM\da\, (\Typd PM\da\, d\, p)\, (\delta\, p)) \\
    &\hspace{.3cm} \to (j , \upmud PM\da\, d\, \delta\da) \equiv \\
    &\hspace{.8cm} \upmu\alg_{m_2}\, (\fst i)\, (\fst c)\, (\snd c)\, \delta\, (\snd i)\, (j \,, d)\, \\
    &\hspace{1.2cm} (\lambda p \to (\Typd M\da, (\fst d) p \,, \snd d\, p)\,, \delta\da\, p)
  \end{align*}
  where we have set
  \begin{align*}
    PM &= \Pb M\, (\Idxd M\da) \\
    PM\da &= \Pbd M\da\, (\lambda\, j\, k \to j \equiv k)
  \end{align*}
  to simplify the notation.

  Now, we may take $e_0'$ to be the identity, since $e_1$ is the
  identity.  It therefore remains to construct the equivalence $e_1'$
  of type
  \[ (i : \Idx M_2) \to \Idxd M\da_2\, i \simeq X_2\, i \] and check
  the two required equations.  We claim that it in fact suffices to
  construct a \emph{map}
  \[ e : (i : \Idx M_2) \to \Idxd M\da_2\, i \to X_2\, i \] and that any
  such map is necessarily an equivalence.  This follows from the fact
  that both $\Idxd M\da_2$ and $X_2$ are multiplicative relations.
  The former by Theorem \ref{thm:slice-alg} and the latter by
  assumption.

  Now, unfolding all the definitions and eliminating the redundancies,
  we find that the map $e$ depends on the data of a tree
  $\sigma : \Cns M_1\, (i,j,c,\nu)$ where $(i,j,c,\nu) : \Idx M_1$, a
  decoration $\phi$ of the nodes of this tree in the family
  $\Idxd M\da_1$, a dependent tree $\sigma\da$ living over $\sigma$
  and a proof $\phi\da$ that the typing function of $\sigma\da$ agrees
  with the data determined by $\phi$ (the situation is analogous to
  that encountered in the proof of Theorem \ref{thm:slice-alg}).  We
  may therefore proceed by simultaneous induction on $\sigma$ and
  $\sigma\da$.
  
  When $\sigma = \lf (i , j)$ and $\sigma\da = \lf (j , \refl)$, we
  must produce an element of $X_2$ of type:
  \[ X_2 (i_s , j_s , \lf (i , j) , \phi) \]
  where
  \begin{align*}
    i_s &= (i \,, j \,, \upeta\, M\, i \,, \etadec j) \\
    j_s &= (j \,, \refl\, , \upetad\, M\da\, j \, , \etadecd \refl) 
  \end{align*}
  on the other hand, we \emph{have} an element
  \begin{align*}
    &x_2 : X_2\, (i_s \,, (\upeta\alg_{m_2} i_s\, (\lf (i , j))\, \phi) \,, \lf (i , j) \,, \phi) \\
    &x_2 = \snd (\ctr (m_2\, (\lf (i \,, x))\, \phi)) 
  \end{align*}
  since $\upeta\alg_{m_2}$ is defined using the multiplicativity of the
  relation $X_2$.  But the term $s\, (i \,, j)\, (j \,, \refl)$
  obtained from the hypothesis $s$ now gives
  \[ j_s \equiv \upeta\alg_{m_2} i_s\, (\lf (i , j))\, \phi \] and we
  so we obtain the desired result by transporting $x_2$ along this
  equality.

  Before moving on to the inductive case of a node, let us pause to
  anticipate how we intend to prove the equations $s'$ and $t'$, as
  this will have serious consequences for how we proceed.  These
  equations will now be over the equivalence $e_1'$ which we are in
  the process of constructing.  Specifically, they take the form
  \begin{align*}
    &s' : (i : \Idx PM_1)\, (j : \Idxd PM\da_1 i) \\
    &\hspace{.3cm} \to e_1' (i , \upeta PM_1 i)\, (j , \upetad PM\da_1\, j) \equiv \\
    &\hspace{1.2cm} \upeta\alg_{m_3}\, (\fst i)\, (\snd i) \\
    \\
    &t' : (i : \Idx PM_1)\, (c : \Cns PM_1 i) \\
    &\hspace{.3cm} \to (\delta : \Pos PM_1\, c) \to \Cns PM_1\, (\Typ PM_1\, c\, p) \\
    &\hspace{.3cm} \to (j : \Idxd PM\da_1\, i) (d : \Cnsd PM\da_1\, j\, c) \\
    &\hspace{.3cm} \to (\delta\da : (p : \Pos PM_1\, c)\\
    &\hspace{1.2cm} \to \Cnsd PM\da_1\, (\Typd PM\da_1\, d\, p)\, (\delta\, p)) \\
    &\hspace{.3cm} \to e_1' (i , \upmu PM_1\, c\, \delta)\, (j , \upmud PM\da_1\, d\, \delta\da) \equiv \\
    &\hspace{.8cm} \upmu\alg_{m_3}\, (\fst i)\, (\fst c)\, (\snd c)\, \delta\, (\snd i)\, (j \,, d)\, \\
    &\hspace{1.2cm} (\lambda p \to (\Typd M_1\da, (\fst d) p \,, \snd d\, p)\,, \delta\da\, p)
  \end{align*}
  where now each of monads have advanced by a single slice
  \begin{align*}
    PM_1 &= \Pb M_1\, (\Idxd M_1\da) \\
    PM\da_1 &= \Pbd M\da_1\, (\lambda\, j\, k \to j \equiv k)
  \end{align*}
  Furthermore, the left side of each equality now includes an
  application of the equivalence $e_1'$, and the right side uses the
  unit and multiplicative operators $\upeta\alg_{m_3}$ and
  $\upmu\alg_{m_3}$ corresponding to the fact that the \emph{next
    family} $X_3$ is also multiplicative.

  What this means is that, if we want to ensure that the equivalence
  $e_1'$ sends the required elements to applications of the unit
  $\upeta\alg_{m_3}$ and multiplication $\upmu\alg_{m_3}$ functions,
  we will need to \emph{use} these functions in the definition of
  $e_1'$ and furthermore, we need to use them \emph{both}.  But since
  the unit case $\upeta\alg_{m_3}$ in the next dimension corresponds
  to a \emph{corolla}, that is, a tree with a single node in the
  present dimension, we will need to now make a case split depending
  on whether or not the node in the tree $\sigma$ we are recursing on
  has descendants or not.  This is possible as soon as the monad $M$
  we are considering is \emph{finitary} in the sense that the type of
  positions is merely equivalent to finite type.  In this case, the
  the property of a tree being a corolla becomes decidable, and so we
  can make the required case split.  This is not a problem for our
  intended application since it is easily checked that the identity
  monad has this property and, moreover, that it is inherited both by
  pulling back and slicing.  Consequently, we will freely proceed now
  under this hypothesis.

  Now, returning to the definition of our equivalence $e_1'$.  We are
  in the inductive case so that we have
  $\sigma = \nd (c \,, \nu)\, \delta\, \epsilon$ and
  $\sigma\da = \nd (c\da \,, \nu\da)\, \delta\da\, \epsilon\da$. Our
  goal is to produce an element of type
  \[ X_2 (i_s , j_s , \nd (c \,, \nu)\, \delta\, \epsilon , \phi) \]
  where now
  \begin{align*}
    i_s &= (i \,, j \,, \upmu\, PM\, (c \,, \nu)\, \delta) \\
    j_s &= (j \,, \refl \,, \upmud\, PM\da\, (c\da \,, \nu\da)\, \delta\da) 
  \end{align*}
  
  We now make a case distinction based on whether the tree $\sigma$ is
  a corolla or not.  In case that it is, one can prove equalities
  \begin{align*}
    &u : (i \,, j \,, \upmu\, PM\, (c \,, \nu)\, \delta) \equiv (i \,, j \,, c \,, \nu) \\
    &v : (j \,, \refl \,, \upmud\, PM\da\, (c\da \,, \nu\da)\, \delta\da) \equiv \phi\, (\inl \ttt) 
  \end{align*}
  But then the result follows from transporting the term
  \[ \upeta\alg_{m_3}\, (i \,, j \,, c \,, \nu)\, (\phi\, (\inl \ttt)) \]
  in the fibration $X_2$ along the equalities $u$ and $v$.

  If $\sigma$ is \emph{not} a corolla, but rather has proper
  descendants, then we proceed as follows: by appealing to the
  induction hypothesis, we obtain a family of elements of $X_2$
  parameterized by the positions $p : \Pos M\, c$.  These assemble,
  together with the \emph{witness} for the binary multiplication of
  $c\da$ and $\delta\da$ under $\upmu\alg_{x_2}$, into the arguments
  for $\upmu\alg_{x_3}$, which has the correct type up to a transport
  along the equality given by our hypothesis $t$.

  This completes the definition of $e_1'$ and, as the reader can see,
  we have thus achieved our goal of using the multiplicative operators
  $\upeta\alg_{m_3}$ and $\upmu\alg_{m_3}$ in the construction of the
  required equivalence.  It remains to check the equations $s'$ and
  $t'$ above, a long calculation which we will not reproduce here.  It
  is not hard to see that, up to some path algebra, $s'$ is by
  definition.  Verifying $t'$ is slightly more involved: in this case,
  one must proceed by induction on the trees occurring in the
  arguments $c$ and $c\da$, again splitting into three cases: that of
  a leaf, a corolla, and a tree with at least 2 nodes.  Additionally,
  during the course of the induction, one uses that the operators
  $\upeta\alg_{m_3}$ and $\upmu\alg_{m_3}$ are \emph{themselves}
  associative and unital under the assumption that the opetopic type
  $X$ was fibrant.
\end{proof}

%%% Local Variables:
%%% mode: latex
%%% TeX-master: "types-are-grpds-ext"
%%% End:
